# Supplementary material for: Geometric Relational Embeddings
Source: arXiv:2409.15369 source file (2024-09-18)
Supplement: Supplementary file 23 [file figs-wiki-talk-vi.tex]

\begin{figure}
  \subfloat[Degree distribution]
  {\includegraphics[width=\textwidth]{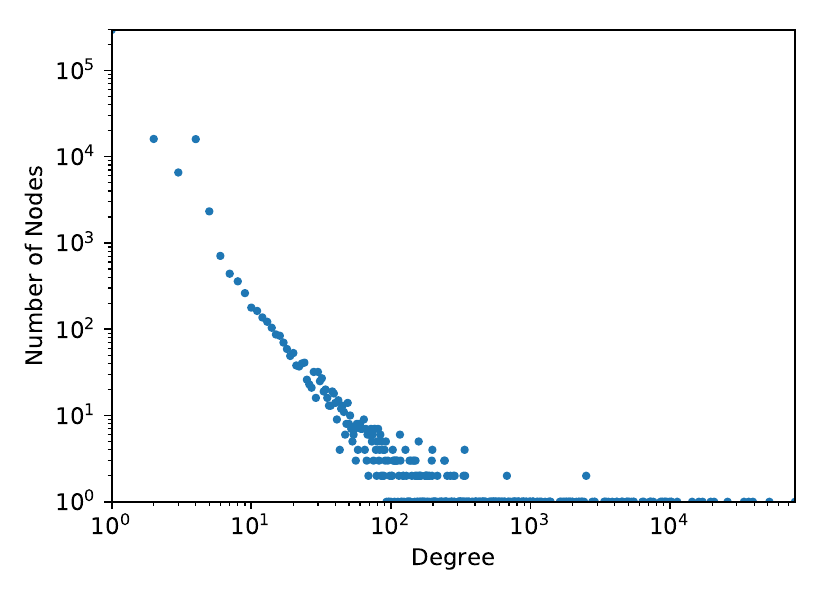}} \\
  \subfloat[Indegree distribution]
  {\includegraphics[width=\textwidth]{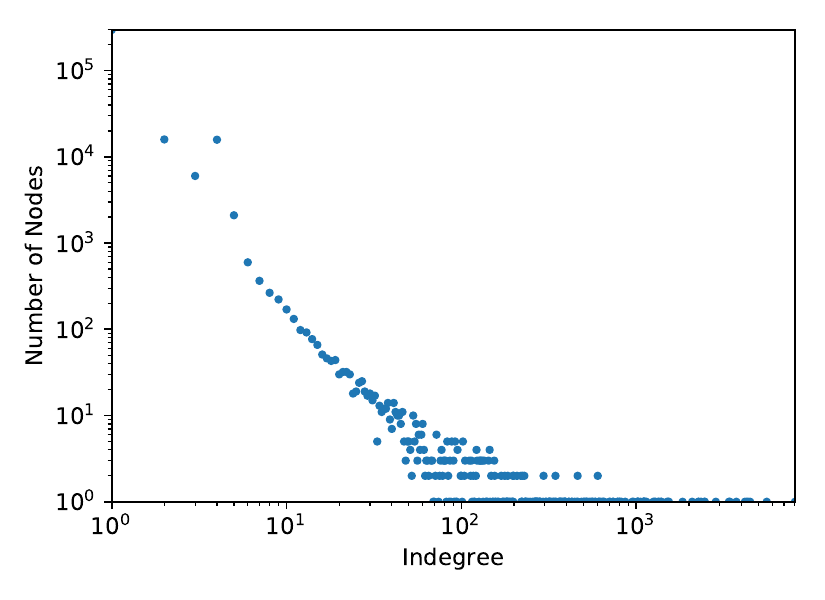}} \\
\end{figure}

\begin{figure}
  \ContinuedFloat \phantomcaption
  \subfloat[Outdegree distribution]
  {\includegraphics[width=\textwidth]{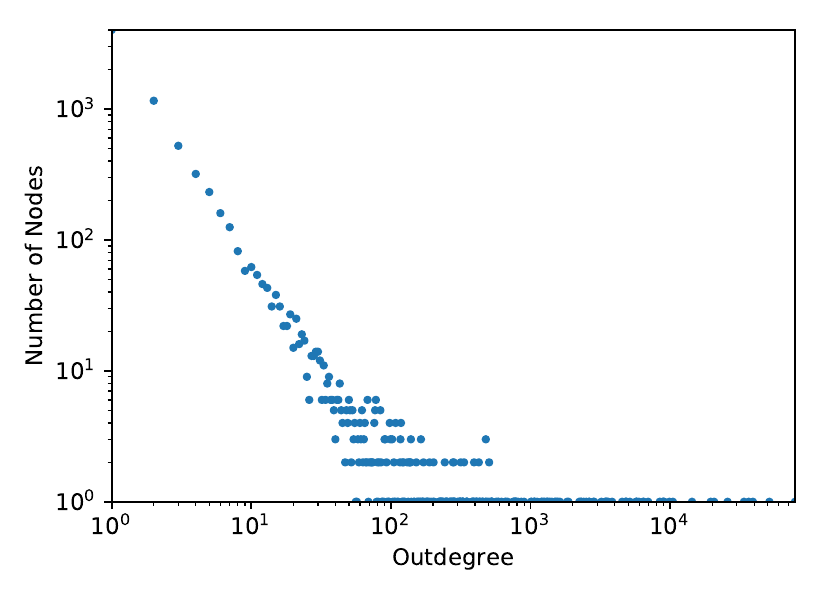}} \\
  \subfloat[Coreness distribution\label{fig_coreness_dist_wiki_talk_vi}]  
  {\includegraphics[width=\textwidth]{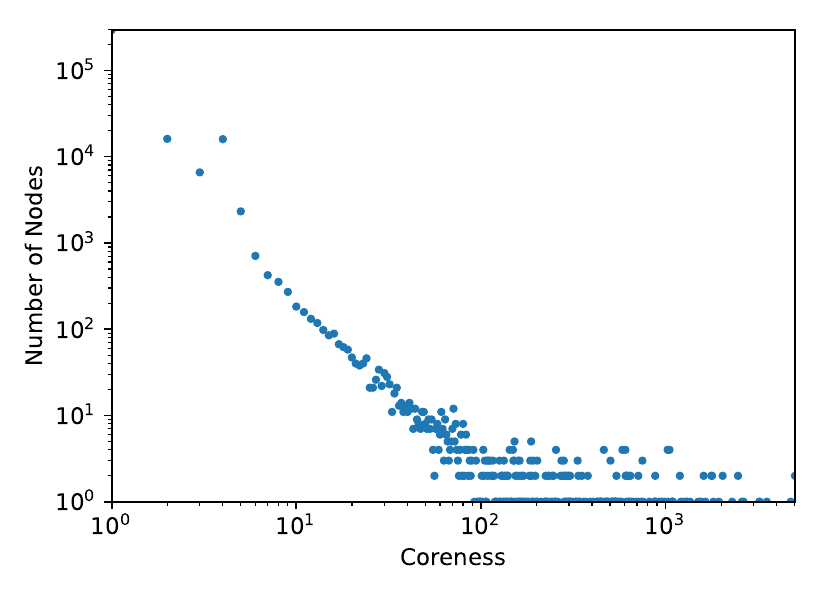}} \\
\end{figure}

\begin{figure}
  \ContinuedFloat \phantomcaption
  \subfloat[Local clustering coefficient distribution]
  {\includegraphics[width=\textwidth]{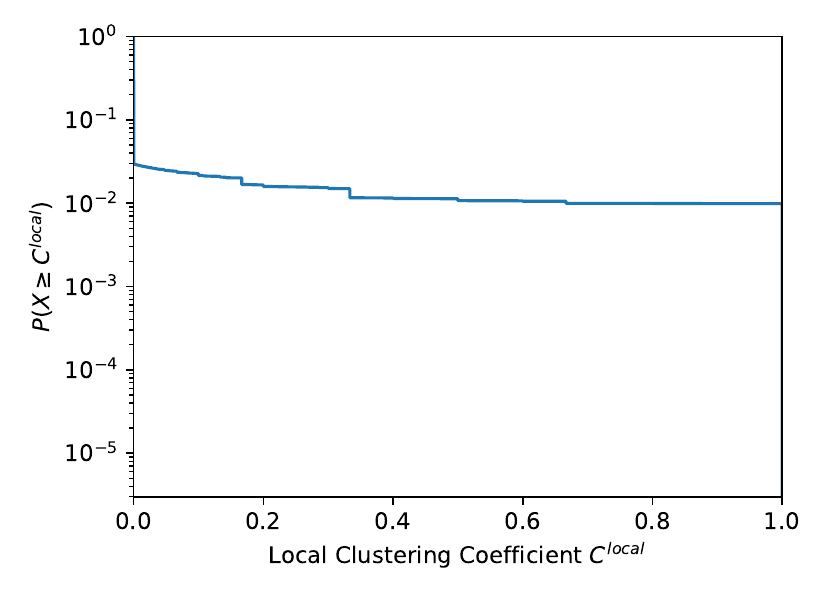}} \\
  \subfloat[PageRank distribution]
  {\includegraphics[width=\textwidth]{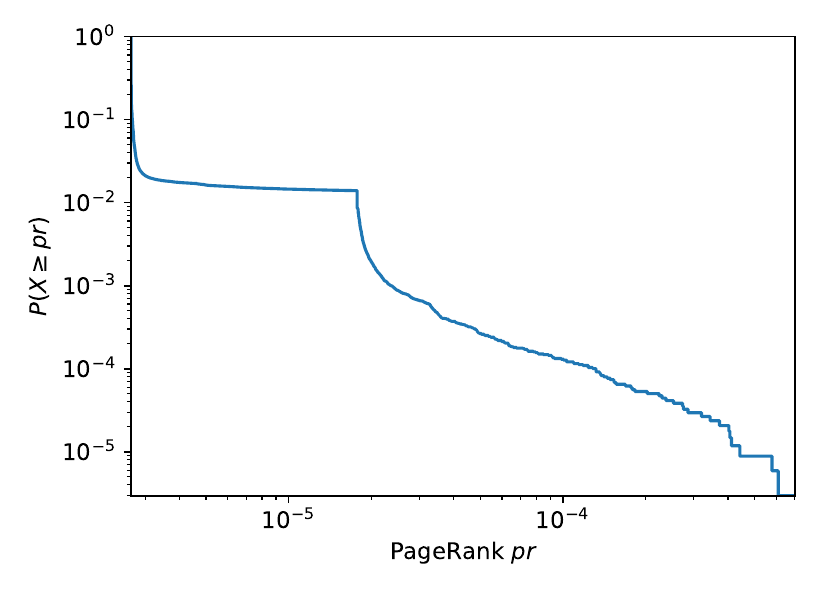}} 
  \caption{The base feature distribution of the Wiki-talk-vi network.}
  \label{fig_feature_dist_wiki_talk_vi}
\end{figure}
\clearpage
